# Supplementary material for: Does Image Anonymization Impact Computer Vision Training?
Source: arXiv:2306.05135 source file (2023-06-08)
Supplement: Supplementary file 1 [file appendix.tex]

\section{Additional Results}

\subsection{Cityscapes All Metrics}
\Cref{tab:cityscapes_full}, \Cref{tab:keypoint_COCO_full}, and \Cref{tab:bdd100k_full} includes all quantitative metrics for Cityscapes, COCO, and BDD100k.

\begin{table*}

    \begin{center}
        \caption{
            Instance segmentation AP on the Cityscapes \cite{cityscapes} validation set with a Mask R-CNN \cite{He2017} \href{https://github.com/facebookresearch/detectron2/blob/main/configs/Cityscapes/mask_rcnn_R_50_FPN.yaml}{R-50 FPN}.
            \textbf{HM}=Histogram matching.
            \textbf{HM-LO}=Histogram matching via Latent Optimization.
            }
        \label{tab:cityscapes_full}
        \resizebox{\linewidth}{!}{
        \begin{tabular}{cccccccccccc}
            \cmidrule[\heavyrulewidth]{2-12}
            &Anonymization Method & AP $\uparrow$ & AP@50 $\uparrow$ & AP$_\text{person}$ & AP$_\text{bus}$ & AP$_\text{bicycle}$ & AP$_\text{car}$ & AP$_\text{motorcycle}$ & AP$_\text{rider}$ & AP$_\text{train}$ & AP$_\text{truck}$ \\
            &Original & $36.7 \pm 0.1$ $(\Delta)$& $62.8 \pm 0.2$ $(\Delta)$& $35.0 \pm 0.2$ $(\Delta)$& $57.6 \pm 0.6$ $(\Delta)$& $23.6 \pm 0.2$ $(\Delta)$& $53.6 \pm 0.0$ $(\Delta)$& $21.9 \pm 0.1$ $(\Delta)$& $28.8 \pm 0.2$ $(\Delta)$& $37.2 \pm 0.4$ $(\Delta)$& $36.1 \pm 0.4$ $(\Delta)$\\
            \cmidrule{2-12}
            \parbox[t]{2mm}{\multirow{3}{*}{\rotatebox[origin=c]{90}{Face}}}& Blur & $36.4 \pm 0.2$ (-0.3) & $62.5 \pm 0.2$ (-0.3) & $34.9 \pm 0.1$ (-0.1) & $\mathbf{58.0} \pm 0.5$ (0.4) & $\mathbf{23.3} \pm 0.1$ (-0.3) & $53.1 \pm 0.1$ (-0.5) & $20.8 \pm 0.5$ (-1.1) & $28.6 \pm 0.1$ (-0.2) & $37.0 \pm 1.3$ (-0.2) & $35.5 \pm 0.5$ (-0.6) \\
            &Mask-out & $\mathbf{36.7} \pm 0.2$ (0.0) & $\mathbf{63.1} \pm 0.2$ (0.3) & $34.9 \pm 0.1$ (-0.1) & $57.5 \pm 0.5$ (-0.1) & $23.2 \pm 0.2$ (-0.4) & $53.2 \pm 0.0$ (-0.4) & $21.4 \pm 0.1$ (-0.5) & $28.7 \pm 0.1$ (-0.1) & $\mathbf{39.5} \pm 0.2$ (2.3) & $35.5 \pm 0.3$ (-0.6) \\
            &Realistic & $36.6 \pm 0.1$ (-0.1) & $62.8 \pm 0.3$ (0.0) & $\mathbf{35.0} \pm 0.1$ (0.0) & $57.2 \pm 0.3$ (-0.4) & $23.2 \pm 0.2$ (-0.4) & $\mathbf{53.4} \pm 0.1$ (-0.2) & $\mathbf{21.7} \pm 0.3$ (-0.2) & $\mathbf{28.8} \pm 0.0$ (0.0) & $36.6 \pm 1.2$ (-0.6) & $\mathbf{36.7} \pm 0.5$ (0.6) \\
            \cmidrule{2-12}
            \parbox[t]{2mm}{\multirow{5}{*}{\rotatebox[origin=c]{90}{Body}}}&Blur & $31.4 \pm 0.2$ (-5.3) & $54.5 \pm 0.4$ (-8.3) & $2.1 \pm 0.1$ (-32.9) & $56.7 \pm 0.6$ (-0.9) & $22.7 \pm 0.1$ (-0.9) & $52.9 \pm 0.1$ (-0.7) & $20.9 \pm 0.2$ (-1.0) & $25.9 \pm 0.2$ (-2.9) & $34.4 \pm 0.5$ (-2.8) & $36.0 \pm 0.7$ (-0.1) \\
            &Mask-out & $31.2 \pm 0.1$ (-5.5) & $53.2 \pm 0.1$ (-9.6) & $0.7 \pm 0.1$ (-34.3) & $55.6 \pm 0.4$ (-2.0) & $22.9 \pm 0.2$ (-0.7) & $52.9 \pm 0.1$ (-0.7) & $21.7 \pm 0.7$ (-0.2) & $25.3 \pm 0.2$ (-3.5) & $35.5 \pm 0.5$ (-1.7) & $35.1 \pm 0.3$ (-1.0) \\
            &Realistic & $34.6 \pm 0.1$ (-2.1) & $59.0 \pm 0.3$ (-3.8) & $20.3 \pm 0.2$ (-14.7) & $\mathbf{58.5} \pm 0.2$ (0.9) & $\mathbf{23.2} \pm 0.1$ (-0.4) & $\mathbf{53.4} \pm 0.1$ (-0.2) & $21.2 \pm 0.2$ (-0.7) & $27.9 \pm 0.5$ (-0.9) & $\mathbf{36.1} \pm 1.5$ (-1.1) & $35.8 \pm 0.6$ (-0.3) \\
            &Realistic + HM & $34.3 \pm 0.2$ (-2.4) & $58.9 \pm 0.2$ (-3.9) & $21.3 \pm 0.3$ (-13.7) & $57.9 \pm 0.2$ (0.3) & $22.8 \pm 0.1$ (-0.8) & $\mathbf{53.4} \pm 0.1$ (-0.2) & $22.0 \pm 0.2$ (0.1) & $27.6 \pm 0.1$ (-1.2) & $34.0 \pm 1.1$ (-3.2) & $35.7 \pm 0.2$ (-0.4) \\
            & Realistic + HM-LO & $\mathbf{34.8} \pm 0.2$ (-1.9) & $\mathbf{60.0} \pm 0.3$ (-2.8) & $\mathbf{21.5} \pm 0.1$ (-13.5) & $57.7 \pm 0.8$ (0.1) & $\mathbf{23.2} \pm 0.2$ (-0.4) & $53.2 \pm 0.0$ (-0.4) & $\mathbf{22.2} \pm 0.3$ (0.3) & $\mathbf{28.1} \pm 0.1$ (-0.7) & $34.9 \pm 1.4$ (-2.3) & $\mathbf{37.3} \pm 0.7$ (1.2) \\
            \cmidrule[\heavyrulewidth]{2-12}
        \end{tabular}}
        \end{center}
        
\end{table*}
\begin{table*}
    \begin{center}
        \caption{
            Keypoint (Kp.) AP on the COCO \cite{Lin2014COCO} validation set with a Keypoint \href{https://github.com/facebookresearch/detectron2/blob/main/configs/COCO-Keypoints/keypoint_rcnn_R_50_FPN_3x.yaml}{R-50 FPN}  R-CNN  \cite{He2017}.
            }
        \label{tab:keypoint_COCO_full}
        \resizebox{\linewidth}{!}{
        \begin{tabular}{ccccccccccccc}
            \cmidrule[\heavyrulewidth]{2-13}
            & Anonymization Method & Box AP $\uparrow$ & Box AP@50 $\uparrow$ & Box AP@75 $\uparrow$ & Box $\text{AP}_{l}$ $\uparrow$ & Box $\text{AP}_{m}$ $\uparrow$ & Box $\text{AP}_{s}$ $\uparrow$ & Kp. AP $\uparrow$ & Kp. AP@50 $\uparrow$ & Kp. AP@75 $\uparrow$ & Kp. $\text{AP}_{l}$ $\uparrow$ & Kp. $\text{AP}_{m}$ $\uparrow$ \\
            & Original & $55.7 \pm 0.0$ $(\Delta)$& $83.3 \pm 0.0$ $(\Delta)$& $60.7 \pm 0.1$ $(\Delta)$& $73.0 \pm 0.1$ $(\Delta)$& $62.9 \pm 0.1$ $(\Delta)$& $37.8 \pm 0.1$ $(\Delta)$& $65.2 \pm 0.0$ $(\Delta)$& $86.3 \pm 0.2$ $(\Delta)$& $71.1 \pm 0.2$ $(\Delta)$& $73.0 \pm 0.0$ $(\Delta)$& $61.2 \pm 0.1$  $(\Delta)$\\
            \cmidrule{2-13}
            \parbox[t]{2mm}{\multirow{4}{*}{\rotatebox[origin=c]{90}{Face}}}& Blur & $50.3 \pm 0.2$ (-5.4) & $77.0 \pm 0.2$ (-6.3) & $54.6 \pm 0.1$ (-6.1) & $67.8 \pm 0.4$ (-5.2) & $52.3 \pm 0.2$ (-10.6) & $37.1 \pm 0.0$ (-0.7) & $53.5 \pm 0.2$ (-11.7) & $74.5 \pm 0.4$ (-11.8) & $57.6 \pm 0.2$ (-13.5) & $63.5 \pm 0.3$ (-9.5) & $48.6 \pm 0.1$ (-12.6) \\
            &Mask-out & $49.9 \pm 0.2$ (-5.8) & $76.6 \pm 0.2$ (-6.7) & $54.1 \pm 0.3$ (-6.6) & $66.9 \pm 0.6$ (-6.1) & $52.3 \pm 0.1$ (-10.6) & $36.8 \pm 0.1$ (-1.0) & $52.0 \pm 0.3$ (-13.2) & $73.5 \pm 0.3$ (-12.8) & $56.2 \pm 0.4$ (-14.9) & $61.4 \pm 0.3$ (-11.6) & $47.7 \pm 0.2$ (-13.5) \\
            &Realistic & $54.3 \pm 0.1$ (-1.4) & $81.7 \pm 0.1$ (-1.6) & $59.0 \pm 0.1$ (-1.7) & $\mathbf{72.7} \pm 0.1$ (-0.3) & $60.0 \pm 0.1$ (-2.9) & $37.3 \pm 0.2$ (-0.5) & $60.6 \pm 0.1$ (-4.6) & $\mathbf{82.9} \pm 0.3$ (-3.4) & $65.9 \pm 0.1$ (-5.2) & $69.9 \pm 0.1$ (-3.1) & $\mathbf{56.1} \pm 0.2$ (-5.1) \\
            &Realistic refined & $\mathbf{54.4} \pm 0.0$ (-1.3) & $\mathbf{81.8} \pm 0.1$ (-1.5) & $\mathbf{59.1} \pm 0.1$ (-1.6) & $\mathbf{72.7} \pm 0.1$ (-0.3) & $\mathbf{60.1} \pm 0.2$ (-2.8) & $\mathbf{37.5} \pm 0.1$ (-0.3) & $\mathbf{60.8} \pm 0.2$ (-4.4) & $\mathbf{82.9} \pm 0.2$ (-3.4) & $\mathbf{66.2} \pm 0.4$ (-4.9) & $\mathbf{70.2} \pm 0.1$ (-2.8) & $\mathbf{56.1} \pm 0.3$ (-5.1) \\
            \cmidrule{2-13}
            \parbox[t]{2mm}{\multirow{3}{*}{\rotatebox[origin=c]{90}{Body}}}&Blur & $17.8 \pm 0.0$ (-37.9) & $35.1 \pm 0.1$ (-48.2) & $16.3 \pm 0.1$ (-44.4) & $2.6 \pm 0.1$ (-70.4) & $10.5 \pm 0.1$ (-52.4) & $33.3 \pm 0.1$ (-4.5) & $4.4 \pm 0.1$ (-60.8) & $9.1 \pm 0.2$ (-77.2) & $3.7 \pm 0.1$ (-67.4) & $0.4 \pm 0.1$ (-72.6) & $10.4 \pm 0.1$ (-50.8) \\
            &Mask-out & $17.4 \pm 0.1$ (-38.3) & $34.5 \pm 0.1$ (-48.8) & $15.5 \pm 0.2$ (-45.2) & $2.1 \pm 0.1$ (-70.9) & $10.6 \pm 0.2$ (-52.3) & $32.5 \pm 0.1$ (-5.3) & $2.0 \pm 0.1$ (-63.2) & $4.9 \pm 0.2$ (-81.4) & $1.4 \pm 0.1$ (-69.7) & $0.1 \pm 0.1$ (-72.9) & $4.1 \pm 0.1$ (-57.1) \\
            & Realistic & $\mathbf{24.0} \pm 0.1$ (-31.7) & $\mathbf{46.1} \pm 0.2$ (-37.2) & $\mathbf{22.4} \pm 0.1$ (-38.3) & $\mathbf{8.2} \pm 0.3$ (-64.8) & $\mathbf{26.4} \pm 0.3$ (-36.5) & $\mathbf{34.1} \pm 0.1$ (-3.7) & $\mathbf{15.6} \pm 0.1$ (-49.6) & $\mathbf{29.4} \pm 0.2$ (-56.9) & $\mathbf{14.2} \pm 0.1$ (-56.9) & $\mathbf{13.0} \pm 0.1$ (-60.0) & $\mathbf{22.5} \pm 0.1$ (-38.7) \\
            \cmidrule[\heavyrulewidth]{2-13}
        \end{tabular}}
        \end{center}

\end{table*}

\begin{table*}
    \begin{center}
        \caption{
            Instance segmentation AP on the BDD100K \cite{Yu2020} validation set with a Mask R-CNN \cite{He2017} \href{https://github.com/SysCV/bdd100k-models/blob/0935a8a3eb4c7442efdce2a8ce4b93fbe585be15/ins_seg/configs/ins_seg/mask_rcnn_r50_fpn_3x_ins_seg_bdd100k.py}{R-50 FPN}.
            }
        \label{tab:bdd100k_full}
        \begin{adjustbox}{max width=\textwidth}
        \begin{tabular}{cccccccccccc}
            \cmidrule[\heavyrulewidth]{2-12}
            &Method & AP $\uparrow$ & AP@50 $\uparrow$ & AP$_\text{pedestrian}$ & AP$_\text{bus}$ & AP$_\text{bicycle}$ & AP$_\text{car}$ & AP$_\text{motorcycle}$ & AP$_\text{rider}$ & AP$_\text{train}$ & AP$_\text{truck}$ \\
            & Original & $20.2 \pm 0.2$ & $34.9 \pm 0.4$ & $32.0 \pm 0.0$ & $30.2 \pm 0.2$ & $6.0 \pm 0.3$ & $45.4 \pm 0.1$ & $11.0 \pm 0.9$ & $9.7 \pm 0.3$ & $0.0 \pm 0.0$ & $26.9 \pm 0.4$ \\
            \cmidrule{2-12}
            \parbox[t]{2mm}{\multirow{3}{*}{\rotatebox[origin=c]{90}{Face}}} & Blur & $20.5 \pm 0.1$ (0.3) & $\mathbf{35.9} \pm 0.1$ (1.0) & $\mathbf{31.7} \pm 0.1$ (-0.3) & $30.1 \pm 0.3$ (-0.1) & $\mathbf{6.9} \pm 0.2$ (0.9) & $45.4 \pm 0.1$ (0.0) & $13.8 \pm 1.0$ (2.8) & $\mathbf{9.4} \pm 0.3$ (-0.3) & $0.0 \pm 0.0$ (0.0) & $26.5 \pm 0.2$ (-0.4) \\
            & Mask-out & $20.3 \pm 0.1$ (0.1) & $35.3 \pm 0.3$ (0.4) & $31.4 \pm 0.1$ (-0.6) & $29.9 \pm 0.5$ (-0.3) & $5.8 \pm 0.3$ (-0.2) & $45.5 \pm 0.1$ (0.1) & $14.4 \pm 0.6$ (3.4) & $8.8 \pm 0.4$ (-0.9) & $0.0 \pm 0.0$ (0.0) & $26.3 \pm 0.2$ (-0.6) \\
            & Realistic & $\mathbf{20.6} \pm 0.1$ (0.4) & $35.8 \pm 0.3$ (0.9) & $31.6 \pm 0.2$ (-0.4) & $\mathbf{30.7} \pm 0.6$ (0.5) & $6.7 \pm 0.4$ (0.7) & $\mathbf{45.6} \pm 0.1$ (0.2) & $\mathbf{14.7} \pm 0.7$ (3.7) & $8.7 \pm 0.2$ (-1.0) & $0.0 \pm 0.0$ (0.0) & $\mathbf{26.7} \pm 0.0$ (-0.2) \\
            \cmidrule{2-12}
            \parbox[t]{2mm}{\multirow{4}{*}{\rotatebox[origin=c]{90}{Body}}} & Blur & $15.4 \pm 0.1$ (-4.8) & $26.3 \pm 0.2$ (-8.6) & $0.5 \pm 0.0$ (-31.5) & $29.5 \pm 0.6$ (-0.7) & $5.4 \pm 0.2$ (-0.6) & $\mathbf{45.6} \pm 0.0$ (0.2) & $12.1 \pm 0.9$ (1.1) & $4.2 \pm 0.3$ (-5.5) & $0.0 \pm 0.0$ (0.0) & $25.9 \pm 0.6$ (-1.0) \\
            & Mask-out & $15.3 \pm 0.0$ (-4.9) & $25.5 \pm 0.1$ (-9.4) & $0.0 \pm 0.0$ (-32.0) & $\mathbf{30.8} \pm 0.2$ (0.6) & $5.5 \pm 0.2$ (-0.5) & $45.5 \pm 0.1$ (0.1) & $10.9 \pm 0.2$ (-0.1) & $3.9 \pm 0.5$ (-5.8) & $0.0 \pm 0.0$ (0.0) & $\mathbf{26.0} \pm 0.4$ (-0.9) \\
            & Realistic & $\mathbf{17.0} \pm 0.1$ (-3.2) & $\mathbf{28.9} \pm 0.4$ (-6.0) & $\mathbf{12.8} \pm 0.1$ (-19.2) & $29.7 \pm 0.4$ (-0.5) & $\mathbf{6.7} \pm 0.3$ (0.7) & $45.2 \pm 0.2$ (-0.2) & $10.3 \pm 0.6$ (-0.7) & $\mathbf{5.8} \pm 0.4$ (-3.9) & $0.0 \pm 0.0$ (0.0) & $25.9 \pm 0.4$ (-1.0) \\
            \cmidrule[\heavyrulewidth]{2-12}
        \end{tabular}
        \end{adjustbox}
        \end{center}
\end{table*}

\subsection{COCO Instance Segmentation}
\begin{table*}
    \begin{center}
        \caption{
            Instance segmentation AP on the COCO \cite{Lin2014COCO} validation set with a Mask \href{https://github.com/facebookresearch/detectron2/blob/main/configs/COCO-InstanceSegmentation/mask_rcnn_R_50_FPN_3x.yaml}{R-50 FPN}  R-CNN  \cite{He2017}.
            }
            \label{tab:instance_COCO}
        \begin{tabular}{ccccc}
            \cmidrule[\heavyrulewidth]{2-5}
             & Anonymization Method & Box AP $\uparrow$ &  Segm. AP $\uparrow$  & Bbox. AP$_\text{person}$ $\uparrow$ \\
             %\cline{2-4}
             & Original & $40.9 \pm 0.0$ $(\Delta)$ & $37.0 \pm 0.0$ $(\Delta)$ & $55.3 \pm 0.1$ $(\Delta)$\\
            %\hhline{~===}
            \cmidrule{2-5}
            \parbox[t]{2mm}{\multirow{3}{*}{\rotatebox[origin=c]{90}{Face}}} &  Blur & $40.7 \pm 0.0$ (-0.2) & $36.9 \pm 0.1$ (-0.1) & $51.9 \pm 0.1$ (-3.4) \\
            %\cline{2-4}
            & Mask-out & $40.6 \pm 0.1$ (-0.3) & $36.9 \pm 0.0$ (-0.1) & $51.6 \pm 0.1$ (-3.7) \\
            %\cline{2-4}
            & Realistic & $\mathbf{40.8} \pm 0.1$ (-0.1) & $\mathbf{37.0} \pm 0.0$ (0.0) & $\mathbf{54.6} \pm 0.1$ (-0.7) \\
            \cmidrule[\heavyrulewidth]{2-5}
        \end{tabular}
        \end{center}
\end{table*}
\Cref{tab:instance_COCO} includes experimental results training a Mask R-CNN for general instance segmentation on the COCO datasets.
Specifically, we train a  Mask \href{https://github.com/facebookresearch/detectron2/blob/main/configs/COCO-InstanceSegmentation/mask_rcnn_R_50_FPN_3x.yaml}{R-50 FPN} R-CNN.
Note that we follow the experimental details from the Keypoint R-CNN experiment in the main paper.

\subsection{Cityscapes - Ignoring Person Annotations}
\Cref{tab:cityscapes_no_persons} show experimental results for Mask R-CNN \cite{He2017} \href{https://github.com/facebookresearch/detectron2/blob/58e472e076a5d861fdcf773d9254a3664e045bf8/configs/Cityscapes/mask_rcnn_R_50_FPN.yaml}{R-50 FPN} on the Cityscapes dataset \cite{cityscapes} without the person class.
It is important to note that we measure the performance drop to the original dataset with person annotations removed.
\begin{table*}

    \begin{center}
        \caption{
            Instance segmentation AP on the Cityscapes \cite{cityscapes} validation set with a Mask R-CNN \cite{He2017} \href{https://github.com/facebookresearch/detectron2/blob/main/configs/Cityscapes/mask_rcnn_R_50_FPN.yaml}{R-50 FPN}.
            Note that the "person" class is removed from all experiments in this table, including the original dataset.
            }
            \label{tab:cityscapes_no_persons}
        \resizebox{\textwidth}{!}{
        \begin{tabular}{ccccccccccc}
            \cmidrule[\heavyrulewidth]{2-11}
            & Anonymization Method & AP $\uparrow$             & AP@50 $\uparrow$          & AP$_\text{bus}$           & AP$_\text{bicycle}$       & AP$_\text{car}$           & AP$_\text{motorcycle}$    & AP$_\text{rider}$         & AP$_\text{train}$         & AP$_\text{truck}$         \\            
            & Original                  & $30.9 \pm 0.3$          $(\Delta)$  & $52.7 \pm 0.7$            $(\Delta)$& $56.1 \pm 0.3$            $(\Delta)$& $22.2 \pm 0.1$            $(\Delta)$& $51.3 \pm 0.1$            $(\Delta)$& $20.5 \pm 0.3$            $(\Delta)$& $25.9 \pm 0.2$            $(\Delta)$& $36.3 \pm 1.4$            $(\Delta)$& $34.7 \pm 0.8$      $(\Delta)$      \\
            \cmidrule{2-11}
            \parbox[t]{2mm}{\multirow{2}{*}{\rotatebox[origin=c]{90}{Body}}} & Blur                      & $30.4 \pm 0.1$ (-0.5)     & $51.6 \pm 0.1$ (-1.1)     & $56.3 \pm 0.1$ (0.2)      & $21.9 \pm 0.1$ (-0.3)     & $50.7 \pm 0.1$ (-0.6)     & $21.1 \pm 0.2$ (0.6)      & $24.4 \pm 0.2$ (-1.5)     & $35.8 \pm 0.6$ (-0.5)     & $33.3 \pm 0.5$ (-1.4)     \\
            & Mask-out                  & $30.6 \pm 0.2$ (-0.3)     & $51.8 \pm 0.3$ (-0.9)     & $55.3 \pm 0.8$ (-0.8)     & $21.5 \pm 0.0$ (-0.7)     & $51.1 \pm 0.1$ (-0.2)     & $20.7 \pm 0.3$ (0.2)      & $23.7 \pm 0.2$ (-2.2)     & $38.3 \pm 0.6$ (2.0)      & $34.4 \pm 0.6$ (-0.3)     \\
            \cmidrule[\heavyrulewidth]{2-11}
        \end{tabular}}
        \end{center}
\end{table*}

\section{Qualitative Anonymization Examples}
The following figures include qualitative examples from Cityscapes \cite{cityscapes} and BDD100k \cite{Yu2020}.

\begin{itemize}
    \item Cityscapes body: \Cref{fig:cityscapes_random_grid_body0}, \ref{fig:cityscapes_random_grid_body1}, \ref{fig:cityscapes_random_grid_body2}.
    \item Cityscapes Body Histogram matching: \Cref{fig:cityscapes_random_HM_grid0}, \ref{fig:cityscapes_random_HM_grid1}, \ref{fig:cityscapes_random_HM_grid2}.
    \item Cityscapes face: \Cref{fig:cityscapes_random_grid_face0}, \ref{fig:cityscapes_random_grid_face1}, \ref{fig:cityscapes_random_grid_face2}.
    \item BDD100k face: \Cref{fig:bdd100k_random_grid_face0}, \ref{fig:bdd100k_random_grid_face1}, \ref{fig:bdd100k_random_grid_face2}, \ref{fig:bdd100k_random_grid_face3}.
    \item BDD100k body: \Cref{fig:bdd100k_random_grid_body0}, \ref{fig:bdd100k_random_grid_body1}, \ref{fig:bdd100k_random_grid_body2}, \ref{fig:bdd100k_random_grid_body3}.
\end{itemize}
\begin{figure*}[t]
\centering
\begin{subfigure}[t]{0.3333333333333333\textwidth}
\centering
\includegraphics[width=\textwidth]{appendix_figures/cityscapes_random/dp2_body_gaussian/aachen_000072_000019_leftImg8bit.jpg}
\includegraphics[width=\textwidth]{appendix_figures/cityscapes_random/dp2_body_gaussian/aachen_000134_000019_leftImg8bit.jpg}
\includegraphics[width=\textwidth]{appendix_figures/cityscapes_random/dp2_body_gaussian/bochum_000000_037829_leftImg8bit.jpg}
\includegraphics[width=\textwidth]{appendix_figures/cityscapes_random/dp2_body_gaussian/bremen_000203_000019_leftImg8bit.jpg}
\includegraphics[width=\textwidth]{appendix_figures/cityscapes_random/dp2_body_gaussian/cologne_000047_000019_leftImg8bit.jpg}
\includegraphics[width=\textwidth]{appendix_figures/cityscapes_random/dp2_body_gaussian/cologne_000133_000019_leftImg8bit.jpg}
\includegraphics[width=\textwidth]{appendix_figures/cityscapes_random/dp2_body_gaussian/darmstadt_000026_000019_leftImg8bit.jpg}
\caption{Body - Gaussian}
\end{subfigure}%%
\begin{subfigure}[t]{0.3333333333333333\textwidth}
\centering
\includegraphics[width=\textwidth]{appendix_figures/cityscapes_random/dp2_body_maskout/aachen_000072_000019_leftImg8bit.jpg}
\includegraphics[width=\textwidth]{appendix_figures/cityscapes_random/dp2_body_maskout/aachen_000134_000019_leftImg8bit.jpg}
\includegraphics[width=\textwidth]{appendix_figures/cityscapes_random/dp2_body_maskout/bochum_000000_037829_leftImg8bit.jpg}
\includegraphics[width=\textwidth]{appendix_figures/cityscapes_random/dp2_body_maskout/bremen_000203_000019_leftImg8bit.jpg}
\includegraphics[width=\textwidth]{appendix_figures/cityscapes_random/dp2_body_maskout/cologne_000047_000019_leftImg8bit.jpg}
\includegraphics[width=\textwidth]{appendix_figures/cityscapes_random/dp2_body_maskout/cologne_000133_000019_leftImg8bit.jpg}
\includegraphics[width=\textwidth]{appendix_figures/cityscapes_random/dp2_body_maskout/darmstadt_000026_000019_leftImg8bit.jpg}
\caption{Body - Mask Out}
\end{subfigure}%%
\begin{subfigure}[t]{0.3333333333333333\textwidth}
\centering
\includegraphics[width=\textwidth]{appendix_figures/cityscapes_random/dp2_SGA_im288_60M_MMT_kpfix/aachen_000072_000019_leftImg8bit.jpg}
\includegraphics[width=\textwidth]{appendix_figures/cityscapes_random/dp2_SGA_im288_60M_MMT_kpfix/aachen_000134_000019_leftImg8bit.jpg}
\includegraphics[width=\textwidth]{appendix_figures/cityscapes_random/dp2_SGA_im288_60M_MMT_kpfix/bochum_000000_037829_leftImg8bit.jpg}
\includegraphics[width=\textwidth]{appendix_figures/cityscapes_random/dp2_SGA_im288_60M_MMT_kpfix/bremen_000203_000019_leftImg8bit.jpg}
\includegraphics[width=\textwidth]{appendix_figures/cityscapes_random/dp2_SGA_im288_60M_MMT_kpfix/cologne_000047_000019_leftImg8bit.jpg}
\includegraphics[width=\textwidth]{appendix_figures/cityscapes_random/dp2_SGA_im288_60M_MMT_kpfix/cologne_000133_000019_leftImg8bit.jpg}
\includegraphics[width=\textwidth]{appendix_figures/cityscapes_random/dp2_SGA_im288_60M_MMT_kpfix/darmstadt_000026_000019_leftImg8bit.jpg}
\caption{Body - Realistic}
\end{subfigure}%%
\caption{Random anonymization examples from Cityscapes \cite{cityscapes}.
\textbf{HM}=Histogram matching.
\textbf{HM-LO}=Histogram matching via Latent Optimization.
Note that the images are compressed.}
\label{fig:cityscapes_random_grid_body0}
\end{figure*}
\begin{figure*}[t]
\centering
\begin{subfigure}[t]{0.3333333333333333\textwidth}
\centering
\includegraphics[width=\textwidth]{appendix_figures/cityscapes_random/dp2_body_gaussian/dusseldorf_000090_000019_leftImg8bit.jpg}
\includegraphics[width=\textwidth]{appendix_figures/cityscapes_random/dp2_body_gaussian/erfurt_000051_000019_leftImg8bit.jpg}
\includegraphics[width=\textwidth]{appendix_figures/cityscapes_random/dp2_body_gaussian/erfurt_000075_000019_leftImg8bit.jpg}
\includegraphics[width=\textwidth]{appendix_figures/cityscapes_random/dp2_body_gaussian/hamburg_000000_050160_leftImg8bit.jpg}
\includegraphics[width=\textwidth]{appendix_figures/cityscapes_random/dp2_body_gaussian/hanover_000000_025335_leftImg8bit.jpg}
\includegraphics[width=\textwidth]{appendix_figures/cityscapes_random/dp2_body_gaussian/krefeld_000000_003707_leftImg8bit.jpg}
\includegraphics[width=\textwidth]{appendix_figures/cityscapes_random/dp2_body_gaussian/krefeld_000000_007325_leftImg8bit.jpg}
\caption{Body - Gaussian}
\end{subfigure}%%
\begin{subfigure}[t]{0.3333333333333333\textwidth}
\centering
\includegraphics[width=\textwidth]{appendix_figures/cityscapes_random/dp2_body_maskout/dusseldorf_000090_000019_leftImg8bit.jpg}
\includegraphics[width=\textwidth]{appendix_figures/cityscapes_random/dp2_body_maskout/erfurt_000051_000019_leftImg8bit.jpg}
\includegraphics[width=\textwidth]{appendix_figures/cityscapes_random/dp2_body_maskout/erfurt_000075_000019_leftImg8bit.jpg}
\includegraphics[width=\textwidth]{appendix_figures/cityscapes_random/dp2_body_maskout/hamburg_000000_050160_leftImg8bit.jpg}
\includegraphics[width=\textwidth]{appendix_figures/cityscapes_random/dp2_body_maskout/hanover_000000_025335_leftImg8bit.jpg}
\includegraphics[width=\textwidth]{appendix_figures/cityscapes_random/dp2_body_maskout/krefeld_000000_003707_leftImg8bit.jpg}
\includegraphics[width=\textwidth]{appendix_figures/cityscapes_random/dp2_body_maskout/krefeld_000000_007325_leftImg8bit.jpg}
\caption{Body - Mask Out}
\end{subfigure}%%
\begin{subfigure}[t]{0.3333333333333333\textwidth}
\centering
\includegraphics[width=\textwidth]{appendix_figures/cityscapes_random/dp2_SGA_im288_60M_MMT_kpfix/dusseldorf_000090_000019_leftImg8bit.jpg}
\includegraphics[width=\textwidth]{appendix_figures/cityscapes_random/dp2_SGA_im288_60M_MMT_kpfix/erfurt_000051_000019_leftImg8bit.jpg}
\includegraphics[width=\textwidth]{appendix_figures/cityscapes_random/dp2_SGA_im288_60M_MMT_kpfix/erfurt_000075_000019_leftImg8bit.jpg}
\includegraphics[width=\textwidth]{appendix_figures/cityscapes_random/dp2_SGA_im288_60M_MMT_kpfix/hamburg_000000_050160_leftImg8bit.jpg}
\includegraphics[width=\textwidth]{appendix_figures/cityscapes_random/dp2_SGA_im288_60M_MMT_kpfix/hanover_000000_025335_leftImg8bit.jpg}
\includegraphics[width=\textwidth]{appendix_figures/cityscapes_random/dp2_SGA_im288_60M_MMT_kpfix/krefeld_000000_003707_leftImg8bit.jpg}
\includegraphics[width=\textwidth]{appendix_figures/cityscapes_random/dp2_SGA_im288_60M_MMT_kpfix/krefeld_000000_007325_leftImg8bit.jpg}
\caption{Body - Realistic}
\end{subfigure}%%
\caption{Random anonymization examples from Cityscapes \cite{cityscapes}.
\textbf{HM}=Histogram matching.
\textbf{HM-LO}=Histogram matching via Latent Optimization.
Note that the images are compressed.}
\label{fig:cityscapes_random_grid_body1}
\end{figure*}
\begin{figure*}[t]
\centering
\begin{subfigure}[t]{0.3333333333333333\textwidth}
\centering
\includegraphics[width=\textwidth]{appendix_figures/cityscapes_random/dp2_body_gaussian/monchengladbach_000000_000076_leftImg8bit.jpg}
\includegraphics[width=\textwidth]{appendix_figures/cityscapes_random/dp2_body_gaussian/strasbourg_000000_010816_leftImg8bit.jpg}
\includegraphics[width=\textwidth]{appendix_figures/cityscapes_random/dp2_body_gaussian/strasbourg_000000_015764_leftImg8bit.jpg}
\includegraphics[width=\textwidth]{appendix_figures/cityscapes_random/dp2_body_gaussian/stuttgart_000114_000019_leftImg8bit.jpg}
\includegraphics[width=\textwidth]{appendix_figures/cityscapes_random/dp2_body_gaussian/tubingen_000056_000019_leftImg8bit.jpg}
\includegraphics[width=\textwidth]{appendix_figures/cityscapes_random/dp2_body_gaussian/ulm_000001_000019_leftImg8bit.jpg}
\includegraphics[width=\textwidth]{appendix_figures/cityscapes_random/dp2_body_gaussian/weimar_000018_000019_leftImg8bit.jpg}
\caption{Body - Gaussian}
\end{subfigure}%%
\begin{subfigure}[t]{0.3333333333333333\textwidth}
\centering
\includegraphics[width=\textwidth]{appendix_figures/cityscapes_random/dp2_body_maskout/monchengladbach_000000_000076_leftImg8bit.jpg}
\includegraphics[width=\textwidth]{appendix_figures/cityscapes_random/dp2_body_maskout/strasbourg_000000_010816_leftImg8bit.jpg}
\includegraphics[width=\textwidth]{appendix_figures/cityscapes_random/dp2_body_maskout/strasbourg_000000_015764_leftImg8bit.jpg}
\includegraphics[width=\textwidth]{appendix_figures/cityscapes_random/dp2_body_maskout/stuttgart_000114_000019_leftImg8bit.jpg}
\includegraphics[width=\textwidth]{appendix_figures/cityscapes_random/dp2_body_maskout/tubingen_000056_000019_leftImg8bit.jpg}
\includegraphics[width=\textwidth]{appendix_figures/cityscapes_random/dp2_body_maskout/ulm_000001_000019_leftImg8bit.jpg}
\includegraphics[width=\textwidth]{appendix_figures/cityscapes_random/dp2_body_maskout/weimar_000018_000019_leftImg8bit.jpg}
\caption{Body - Mask Out}
\end{subfigure}%%
\begin{subfigure}[t]{0.3333333333333333\textwidth}
\centering
\includegraphics[width=\textwidth]{appendix_figures/cityscapes_random/dp2_SGA_im288_60M_MMT_kpfix/monchengladbach_000000_000076_leftImg8bit.jpg}
\includegraphics[width=\textwidth]{appendix_figures/cityscapes_random/dp2_SGA_im288_60M_MMT_kpfix/strasbourg_000000_010816_leftImg8bit.jpg}
\includegraphics[width=\textwidth]{appendix_figures/cityscapes_random/dp2_SGA_im288_60M_MMT_kpfix/strasbourg_000000_015764_leftImg8bit.jpg}
\includegraphics[width=\textwidth]{appendix_figures/cityscapes_random/dp2_SGA_im288_60M_MMT_kpfix/stuttgart_000114_000019_leftImg8bit.jpg}
\includegraphics[width=\textwidth]{appendix_figures/cityscapes_random/dp2_SGA_im288_60M_MMT_kpfix/tubingen_000056_000019_leftImg8bit.jpg}
\includegraphics[width=\textwidth]{appendix_figures/cityscapes_random/dp2_SGA_im288_60M_MMT_kpfix/ulm_000001_000019_leftImg8bit.jpg}
\includegraphics[width=\textwidth]{appendix_figures/cityscapes_random/dp2_SGA_im288_60M_MMT_kpfix/weimar_000018_000019_leftImg8bit.jpg}
\caption{Body - Realistic}
\end{subfigure}%%
\caption{Random anonymization examples from Cityscapes \cite{cityscapes}.
\textbf{HM}=Histogram matching.
\textbf{HM-LO}=Histogram matching via Latent Optimization.
Note that the images are compressed.}
\label{fig:cityscapes_random_grid_body2}
\end{figure*}

\begin{figure*}[t]
\centering
\begin{subfigure}[t]{0.3333333333333333\textwidth}
\centering
\includegraphics[width=\textwidth]{appendix_figures/cityscapes_random/dp2_face_gaussian/aachen_000072_000019_leftImg8bit.jpg}
\includegraphics[width=\textwidth]{appendix_figures/cityscapes_random/dp2_face_gaussian/aachen_000134_000019_leftImg8bit.jpg}
\includegraphics[width=\textwidth]{appendix_figures/cityscapes_random/dp2_face_gaussian/bochum_000000_037829_leftImg8bit.jpg}
\includegraphics[width=\textwidth]{appendix_figures/cityscapes_random/dp2_face_gaussian/bremen_000203_000019_leftImg8bit.jpg}
\includegraphics[width=\textwidth]{appendix_figures/cityscapes_random/dp2_face_gaussian/cologne_000047_000019_leftImg8bit.jpg}
\includegraphics[width=\textwidth]{appendix_figures/cityscapes_random/dp2_face_gaussian/cologne_000133_000019_leftImg8bit.jpg}
\includegraphics[width=\textwidth]{appendix_figures/cityscapes_random/dp2_face_gaussian/darmstadt_000026_000019_leftImg8bit.jpg}
\caption{Face - Gaussian}
\end{subfigure}%%
\begin{subfigure}[t]{0.3333333333333333\textwidth}
\centering
\includegraphics[width=\textwidth]{appendix_figures/cityscapes_random/dp2_face_maskout/aachen_000072_000019_leftImg8bit.jpg}
\includegraphics[width=\textwidth]{appendix_figures/cityscapes_random/dp2_face_maskout/aachen_000134_000019_leftImg8bit.jpg}
\includegraphics[width=\textwidth]{appendix_figures/cityscapes_random/dp2_face_maskout/bochum_000000_037829_leftImg8bit.jpg}
\includegraphics[width=\textwidth]{appendix_figures/cityscapes_random/dp2_face_maskout/bremen_000203_000019_leftImg8bit.jpg}
\includegraphics[width=\textwidth]{appendix_figures/cityscapes_random/dp2_face_maskout/cologne_000047_000019_leftImg8bit.jpg}
\includegraphics[width=\textwidth]{appendix_figures/cityscapes_random/dp2_face_maskout/cologne_000133_000019_leftImg8bit.jpg}
\includegraphics[width=\textwidth]{appendix_figures/cityscapes_random/dp2_face_maskout/darmstadt_000026_000019_leftImg8bit.jpg}
\caption{Face - Mask Out}
\end{subfigure}%%
\begin{subfigure}[t]{0.3333333333333333\textwidth}
\centering
\includegraphics[width=\textwidth]{appendix_figures/cityscapes_random/dp2_face_fdf128/aachen_000072_000019_leftImg8bit.jpg}
\includegraphics[width=\textwidth]{appendix_figures/cityscapes_random/dp2_face_fdf128/aachen_000134_000019_leftImg8bit.jpg}
\includegraphics[width=\textwidth]{appendix_figures/cityscapes_random/dp2_face_fdf128/bochum_000000_037829_leftImg8bit.jpg}
\includegraphics[width=\textwidth]{appendix_figures/cityscapes_random/dp2_face_fdf128/bremen_000203_000019_leftImg8bit.jpg}
\includegraphics[width=\textwidth]{appendix_figures/cityscapes_random/dp2_face_fdf128/cologne_000047_000019_leftImg8bit.jpg}
\includegraphics[width=\textwidth]{appendix_figures/cityscapes_random/dp2_face_fdf128/cologne_000133_000019_leftImg8bit.jpg}
\includegraphics[width=\textwidth]{appendix_figures/cityscapes_random/dp2_face_fdf128/darmstadt_000026_000019_leftImg8bit.jpg}
\caption{Face - Realistic}
\end{subfigure}%%
\caption{Random anonymization examples from Cityscapes \cite{cityscapes}.
\textbf{HM}=Histogram matching.
\textbf{HM-LO}=Histogram matching via Latent Optimization.
Note that the images are compressed.}
\label{fig:cityscapes_random_grid_face0}
\end{figure*}
\begin{figure*}[t]
\centering
\begin{subfigure}[t]{0.3333333333333333\textwidth}
\centering
\includegraphics[width=\textwidth]{appendix_figures/cityscapes_random/dp2_face_gaussian/dusseldorf_000090_000019_leftImg8bit.jpg}
\includegraphics[width=\textwidth]{appendix_figures/cityscapes_random/dp2_face_gaussian/erfurt_000051_000019_leftImg8bit.jpg}
\includegraphics[width=\textwidth]{appendix_figures/cityscapes_random/dp2_face_gaussian/erfurt_000075_000019_leftImg8bit.jpg}
\includegraphics[width=\textwidth]{appendix_figures/cityscapes_random/dp2_face_gaussian/hamburg_000000_050160_leftImg8bit.jpg}
\includegraphics[width=\textwidth]{appendix_figures/cityscapes_random/dp2_face_gaussian/hanover_000000_025335_leftImg8bit.jpg}
\includegraphics[width=\textwidth]{appendix_figures/cityscapes_random/dp2_face_gaussian/krefeld_000000_003707_leftImg8bit.jpg}
\includegraphics[width=\textwidth]{appendix_figures/cityscapes_random/dp2_face_gaussian/krefeld_000000_007325_leftImg8bit.jpg}
\caption{Face - Gaussian}
\end{subfigure}%%
\begin{subfigure}[t]{0.3333333333333333\textwidth}
\centering
\includegraphics[width=\textwidth]{appendix_figures/cityscapes_random/dp2_face_maskout/dusseldorf_000090_000019_leftImg8bit.jpg}
\includegraphics[width=\textwidth]{appendix_figures/cityscapes_random/dp2_face_maskout/erfurt_000051_000019_leftImg8bit.jpg}
\includegraphics[width=\textwidth]{appendix_figures/cityscapes_random/dp2_face_maskout/erfurt_000075_000019_leftImg8bit.jpg}
\includegraphics[width=\textwidth]{appendix_figures/cityscapes_random/dp2_face_maskout/hamburg_000000_050160_leftImg8bit.jpg}
\includegraphics[width=\textwidth]{appendix_figures/cityscapes_random/dp2_face_maskout/hanover_000000_025335_leftImg8bit.jpg}
\includegraphics[width=\textwidth]{appendix_figures/cityscapes_random/dp2_face_maskout/krefeld_000000_003707_leftImg8bit.jpg}
\includegraphics[width=\textwidth]{appendix_figures/cityscapes_random/dp2_face_maskout/krefeld_000000_007325_leftImg8bit.jpg}
\caption{Face - Mask Out}
\end{subfigure}%%
\begin{subfigure}[t]{0.3333333333333333\textwidth}
\centering
\includegraphics[width=\textwidth]{appendix_figures/cityscapes_random/dp2_face_fdf128/dusseldorf_000090_000019_leftImg8bit.jpg}
\includegraphics[width=\textwidth]{appendix_figures/cityscapes_random/dp2_face_fdf128/erfurt_000051_000019_leftImg8bit.jpg}
\includegraphics[width=\textwidth]{appendix_figures/cityscapes_random/dp2_face_fdf128/erfurt_000075_000019_leftImg8bit.jpg}
\includegraphics[width=\textwidth]{appendix_figures/cityscapes_random/dp2_face_fdf128/hamburg_000000_050160_leftImg8bit.jpg}
\includegraphics[width=\textwidth]{appendix_figures/cityscapes_random/dp2_face_fdf128/hanover_000000_025335_leftImg8bit.jpg}
\includegraphics[width=\textwidth]{appendix_figures/cityscapes_random/dp2_face_fdf128/krefeld_000000_003707_leftImg8bit.jpg}
\includegraphics[width=\textwidth]{appendix_figures/cityscapes_random/dp2_face_fdf128/krefeld_000000_007325_leftImg8bit.jpg}
\caption{Face - Realistic}
\end{subfigure}%%
\caption{Random anonymization examples from Cityscapes \cite{cityscapes}.
\textbf{HM}=Histogram matching.
\textbf{HM-LO}=Histogram matching via Latent Optimization.
Note that the images are compressed.}
\label{fig:cityscapes_random_grid_face1}
\end{figure*}
\begin{figure*}[t]
\centering
\begin{subfigure}[t]{0.3333333333333333\textwidth}
\centering
\includegraphics[width=\textwidth]{appendix_figures/cityscapes_random/dp2_face_gaussian/monchengladbach_000000_000076_leftImg8bit.jpg}
\includegraphics[width=\textwidth]{appendix_figures/cityscapes_random/dp2_face_gaussian/strasbourg_000000_010816_leftImg8bit.jpg}
\includegraphics[width=\textwidth]{appendix_figures/cityscapes_random/dp2_face_gaussian/strasbourg_000000_015764_leftImg8bit.jpg}
\includegraphics[width=\textwidth]{appendix_figures/cityscapes_random/dp2_face_gaussian/stuttgart_000114_000019_leftImg8bit.jpg}
\includegraphics[width=\textwidth]{appendix_figures/cityscapes_random/dp2_face_gaussian/tubingen_000056_000019_leftImg8bit.jpg}
\includegraphics[width=\textwidth]{appendix_figures/cityscapes_random/dp2_face_gaussian/ulm_000001_000019_leftImg8bit.jpg}
\includegraphics[width=\textwidth]{appendix_figures/cityscapes_random/dp2_face_gaussian/weimar_000018_000019_leftImg8bit.jpg}
\caption{Face - Gaussian}
\end{subfigure}%%
\begin{subfigure}[t]{0.3333333333333333\textwidth}
\centering
\includegraphics[width=\textwidth]{appendix_figures/cityscapes_random/dp2_face_maskout/monchengladbach_000000_000076_leftImg8bit.jpg}
\includegraphics[width=\textwidth]{appendix_figures/cityscapes_random/dp2_face_maskout/strasbourg_000000_010816_leftImg8bit.jpg}
\includegraphics[width=\textwidth]{appendix_figures/cityscapes_random/dp2_face_maskout/strasbourg_000000_015764_leftImg8bit.jpg}
\includegraphics[width=\textwidth]{appendix_figures/cityscapes_random/dp2_face_maskout/stuttgart_000114_000019_leftImg8bit.jpg}
\includegraphics[width=\textwidth]{appendix_figures/cityscapes_random/dp2_face_maskout/tubingen_000056_000019_leftImg8bit.jpg}
\includegraphics[width=\textwidth]{appendix_figures/cityscapes_random/dp2_face_maskout/ulm_000001_000019_leftImg8bit.jpg}
\includegraphics[width=\textwidth]{appendix_figures/cityscapes_random/dp2_face_maskout/weimar_000018_000019_leftImg8bit.jpg}
\caption{Face - Mask Out}
\end{subfigure}%%
\begin{subfigure}[t]{0.3333333333333333\textwidth}
\centering
\includegraphics[width=\textwidth]{appendix_figures/cityscapes_random/dp2_face_fdf128/monchengladbach_000000_000076_leftImg8bit.jpg}
\includegraphics[width=\textwidth]{appendix_figures/cityscapes_random/dp2_face_fdf128/strasbourg_000000_010816_leftImg8bit.jpg}
\includegraphics[width=\textwidth]{appendix_figures/cityscapes_random/dp2_face_fdf128/strasbourg_000000_015764_leftImg8bit.jpg}
\includegraphics[width=\textwidth]{appendix_figures/cityscapes_random/dp2_face_fdf128/stuttgart_000114_000019_leftImg8bit.jpg}
\includegraphics[width=\textwidth]{appendix_figures/cityscapes_random/dp2_face_fdf128/tubingen_000056_000019_leftImg8bit.jpg}
\includegraphics[width=\textwidth]{appendix_figures/cityscapes_random/dp2_face_fdf128/ulm_000001_000019_leftImg8bit.jpg}
\includegraphics[width=\textwidth]{appendix_figures/cityscapes_random/dp2_face_fdf128/weimar_000018_000019_leftImg8bit.jpg}
\caption{Face - Realistic}
\end{subfigure}%%
\caption{Random anonymization examples from Cityscapes \cite{cityscapes}.
\textbf{HM}=Histogram matching.
\textbf{HM-LO}=Histogram matching via Latent Optimization.
Note that the images are compressed.}
\label{fig:cityscapes_random_grid_face2}
\end{figure*}

\begin{figure*}[t]
\centering
\begin{subfigure}[t]{0.3333333333333333\textwidth}
\centering
\includegraphics[width=\textwidth]{appendix_figures/cityscapes_random/dp2_SGA_im288_60M_MMT_kpfix/aachen_000072_000019_leftImg8bit.jpg}
\includegraphics[width=\textwidth]{appendix_figures/cityscapes_random/dp2_SGA_im288_60M_MMT_kpfix/aachen_000134_000019_leftImg8bit.jpg}
\includegraphics[width=\textwidth]{appendix_figures/cityscapes_random/dp2_SGA_im288_60M_MMT_kpfix/bochum_000000_037829_leftImg8bit.jpg}
\includegraphics[width=\textwidth]{appendix_figures/cityscapes_random/dp2_SGA_im288_60M_MMT_kpfix/bremen_000203_000019_leftImg8bit.jpg}
\includegraphics[width=\textwidth]{appendix_figures/cityscapes_random/dp2_SGA_im288_60M_MMT_kpfix/cologne_000047_000019_leftImg8bit.jpg}
\includegraphics[width=\textwidth]{appendix_figures/cityscapes_random/dp2_SGA_im288_60M_MMT_kpfix/cologne_000133_000019_leftImg8bit.jpg}
\includegraphics[width=\textwidth]{appendix_figures/cityscapes_random/dp2_SGA_im288_60M_MMT_kpfix/darmstadt_000026_000019_leftImg8bit.jpg}
\caption{Body - Realistic}
\end{subfigure}%%
\begin{subfigure}[t]{0.3333333333333333\textwidth}
\centering
\includegraphics[width=\textwidth]{appendix_figures/cityscapes_random/dp2_SGA_im288_60M_MH_MMT_kpfix/aachen_000072_000019_leftImg8bit.jpg}
\includegraphics[width=\textwidth]{appendix_figures/cityscapes_random/dp2_SGA_im288_60M_MH_MMT_kpfix/aachen_000134_000019_leftImg8bit.jpg}
\includegraphics[width=\textwidth]{appendix_figures/cityscapes_random/dp2_SGA_im288_60M_MH_MMT_kpfix/bochum_000000_037829_leftImg8bit.jpg}
\includegraphics[width=\textwidth]{appendix_figures/cityscapes_random/dp2_SGA_im288_60M_MH_MMT_kpfix/bremen_000203_000019_leftImg8bit.jpg}
\includegraphics[width=\textwidth]{appendix_figures/cityscapes_random/dp2_SGA_im288_60M_MH_MMT_kpfix/cologne_000047_000019_leftImg8bit.jpg}
\includegraphics[width=\textwidth]{appendix_figures/cityscapes_random/dp2_SGA_im288_60M_MH_MMT_kpfix/cologne_000133_000019_leftImg8bit.jpg}
\includegraphics[width=\textwidth]{appendix_figures/cityscapes_random/dp2_SGA_im288_60M_MH_MMT_kpfix/darmstadt_000026_000019_leftImg8bit.jpg}
\caption{Body - Realistic (HM)}
\end{subfigure}%%
\begin{subfigure}[t]{0.3333333333333333\textwidth}
\centering
\includegraphics[width=\textwidth]{appendix_figures/cityscapes_random/dp2_SGA_im288_60M_MMT_sample100_kpfix/aachen_000072_000019_leftImg8bit.jpg}
\includegraphics[width=\textwidth]{appendix_figures/cityscapes_random/dp2_SGA_im288_60M_MMT_sample100_kpfix/aachen_000134_000019_leftImg8bit.jpg}
\includegraphics[width=\textwidth]{appendix_figures/cityscapes_random/dp2_SGA_im288_60M_MMT_sample100_kpfix/bochum_000000_037829_leftImg8bit.jpg}
\includegraphics[width=\textwidth]{appendix_figures/cityscapes_random/dp2_SGA_im288_60M_MMT_sample100_kpfix/bremen_000203_000019_leftImg8bit.jpg}
\includegraphics[width=\textwidth]{appendix_figures/cityscapes_random/dp2_SGA_im288_60M_MMT_sample100_kpfix/cologne_000047_000019_leftImg8bit.jpg}
\includegraphics[width=\textwidth]{appendix_figures/cityscapes_random/dp2_SGA_im288_60M_MMT_sample100_kpfix/cologne_000133_000019_leftImg8bit.jpg}
\includegraphics[width=\textwidth]{appendix_figures/cityscapes_random/dp2_SGA_im288_60M_MMT_sample100_kpfix/darmstadt_000026_000019_leftImg8bit.jpg}
\caption{Body - Realistic (HM-LO)}
\end{subfigure}%%
\caption{Random anonymization examples from Cityscapes \cite{cityscapes}.
\textbf{HM}=Histogram matching.
\textbf{HM-LO}=Histogram matching via Latent Optimization.
Note that the images are compressed.}
\label{fig:cityscapes_random_HM_grid0}
\end{figure*}
\begin{figure*}[t]
\centering
\begin{subfigure}[t]{0.3333333333333333\textwidth}
\centering
\includegraphics[width=\textwidth]{appendix_figures/cityscapes_random/dp2_SGA_im288_60M_MMT_kpfix/dusseldorf_000090_000019_leftImg8bit.jpg}
\includegraphics[width=\textwidth]{appendix_figures/cityscapes_random/dp2_SGA_im288_60M_MMT_kpfix/erfurt_000051_000019_leftImg8bit.jpg}
\includegraphics[width=\textwidth]{appendix_figures/cityscapes_random/dp2_SGA_im288_60M_MMT_kpfix/erfurt_000075_000019_leftImg8bit.jpg}
\includegraphics[width=\textwidth]{appendix_figures/cityscapes_random/dp2_SGA_im288_60M_MMT_kpfix/hamburg_000000_050160_leftImg8bit.jpg}
\includegraphics[width=\textwidth]{appendix_figures/cityscapes_random/dp2_SGA_im288_60M_MMT_kpfix/hanover_000000_025335_leftImg8bit.jpg}
\includegraphics[width=\textwidth]{appendix_figures/cityscapes_random/dp2_SGA_im288_60M_MMT_kpfix/krefeld_000000_003707_leftImg8bit.jpg}
\includegraphics[width=\textwidth]{appendix_figures/cityscapes_random/dp2_SGA_im288_60M_MMT_kpfix/krefeld_000000_007325_leftImg8bit.jpg}
\caption{Body - Realistic}
\end{subfigure}%%
\begin{subfigure}[t]{0.3333333333333333\textwidth}
\centering
\includegraphics[width=\textwidth]{appendix_figures/cityscapes_random/dp2_SGA_im288_60M_MH_MMT_kpfix/dusseldorf_000090_000019_leftImg8bit.jpg}
\includegraphics[width=\textwidth]{appendix_figures/cityscapes_random/dp2_SGA_im288_60M_MH_MMT_kpfix/erfurt_000051_000019_leftImg8bit.jpg}
\includegraphics[width=\textwidth]{appendix_figures/cityscapes_random/dp2_SGA_im288_60M_MH_MMT_kpfix/erfurt_000075_000019_leftImg8bit.jpg}
\includegraphics[width=\textwidth]{appendix_figures/cityscapes_random/dp2_SGA_im288_60M_MH_MMT_kpfix/hamburg_000000_050160_leftImg8bit.jpg}
\includegraphics[width=\textwidth]{appendix_figures/cityscapes_random/dp2_SGA_im288_60M_MH_MMT_kpfix/hanover_000000_025335_leftImg8bit.jpg}
\includegraphics[width=\textwidth]{appendix_figures/cityscapes_random/dp2_SGA_im288_60M_MH_MMT_kpfix/krefeld_000000_003707_leftImg8bit.jpg}
\includegraphics[width=\textwidth]{appendix_figures/cityscapes_random/dp2_SGA_im288_60M_MH_MMT_kpfix/krefeld_000000_007325_leftImg8bit.jpg}
\caption{Body - Realistic (HM)}
\end{subfigure}%%
\begin{subfigure}[t]{0.3333333333333333\textwidth}
\centering
\includegraphics[width=\textwidth]{appendix_figures/cityscapes_random/dp2_SGA_im288_60M_MMT_sample100_kpfix/dusseldorf_000090_000019_leftImg8bit.jpg}
\includegraphics[width=\textwidth]{appendix_figures/cityscapes_random/dp2_SGA_im288_60M_MMT_sample100_kpfix/erfurt_000051_000019_leftImg8bit.jpg}
\includegraphics[width=\textwidth]{appendix_figures/cityscapes_random/dp2_SGA_im288_60M_MMT_sample100_kpfix/erfurt_000075_000019_leftImg8bit.jpg}
\includegraphics[width=\textwidth]{appendix_figures/cityscapes_random/dp2_SGA_im288_60M_MMT_sample100_kpfix/hamburg_000000_050160_leftImg8bit.jpg}
\includegraphics[width=\textwidth]{appendix_figures/cityscapes_random/dp2_SGA_im288_60M_MMT_sample100_kpfix/hanover_000000_025335_leftImg8bit.jpg}
\includegraphics[width=\textwidth]{appendix_figures/cityscapes_random/dp2_SGA_im288_60M_MMT_sample100_kpfix/krefeld_000000_003707_leftImg8bit.jpg}
\includegraphics[width=\textwidth]{appendix_figures/cityscapes_random/dp2_SGA_im288_60M_MMT_sample100_kpfix/krefeld_000000_007325_leftImg8bit.jpg}
\caption{Body - Realistic (HM-LO)}
\end{subfigure}%%
\caption{Random anonymization examples from Cityscapes \cite{cityscapes}.
\textbf{HM}=Histogram matching.
\textbf{HM-LO}=Histogram matching via Latent Optimization.
Note that the images are compressed.}
\label{fig:cityscapes_random_HM_grid1}
\end{figure*}
\begin{figure*}[t]
\centering
\begin{subfigure}[t]{0.3333333333333333\textwidth}
\centering
\includegraphics[width=\textwidth]{appendix_figures/cityscapes_random/dp2_SGA_im288_60M_MMT_kpfix/monchengladbach_000000_000076_leftImg8bit.jpg}
\includegraphics[width=\textwidth]{appendix_figures/cityscapes_random/dp2_SGA_im288_60M_MMT_kpfix/strasbourg_000000_010816_leftImg8bit.jpg}
\includegraphics[width=\textwidth]{appendix_figures/cityscapes_random/dp2_SGA_im288_60M_MMT_kpfix/strasbourg_000000_015764_leftImg8bit.jpg}
\includegraphics[width=\textwidth]{appendix_figures/cityscapes_random/dp2_SGA_im288_60M_MMT_kpfix/stuttgart_000114_000019_leftImg8bit.jpg}
\includegraphics[width=\textwidth]{appendix_figures/cityscapes_random/dp2_SGA_im288_60M_MMT_kpfix/tubingen_000056_000019_leftImg8bit.jpg}
\includegraphics[width=\textwidth]{appendix_figures/cityscapes_random/dp2_SGA_im288_60M_MMT_kpfix/ulm_000001_000019_leftImg8bit.jpg}
\includegraphics[width=\textwidth]{appendix_figures/cityscapes_random/dp2_SGA_im288_60M_MMT_kpfix/weimar_000018_000019_leftImg8bit.jpg}
\caption{Body - Realistic}
\end{subfigure}%%
\begin{subfigure}[t]{0.3333333333333333\textwidth}
\centering
\includegraphics[width=\textwidth]{appendix_figures/cityscapes_random/dp2_SGA_im288_60M_MH_MMT_kpfix/monchengladbach_000000_000076_leftImg8bit.jpg}
\includegraphics[width=\textwidth]{appendix_figures/cityscapes_random/dp2_SGA_im288_60M_MH_MMT_kpfix/strasbourg_000000_010816_leftImg8bit.jpg}
\includegraphics[width=\textwidth]{appendix_figures/cityscapes_random/dp2_SGA_im288_60M_MH_MMT_kpfix/strasbourg_000000_015764_leftImg8bit.jpg}
\includegraphics[width=\textwidth]{appendix_figures/cityscapes_random/dp2_SGA_im288_60M_MH_MMT_kpfix/stuttgart_000114_000019_leftImg8bit.jpg}
\includegraphics[width=\textwidth]{appendix_figures/cityscapes_random/dp2_SGA_im288_60M_MH_MMT_kpfix/tubingen_000056_000019_leftImg8bit.jpg}
\includegraphics[width=\textwidth]{appendix_figures/cityscapes_random/dp2_SGA_im288_60M_MH_MMT_kpfix/ulm_000001_000019_leftImg8bit.jpg}
\includegraphics[width=\textwidth]{appendix_figures/cityscapes_random/dp2_SGA_im288_60M_MH_MMT_kpfix/weimar_000018_000019_leftImg8bit.jpg}
\caption{Body - Realistic (HM)}
\end{subfigure}%%
\begin{subfigure}[t]{0.3333333333333333\textwidth}
\centering
\includegraphics[width=\textwidth]{appendix_figures/cityscapes_random/dp2_SGA_im288_60M_MMT_sample100_kpfix/monchengladbach_000000_000076_leftImg8bit.jpg}
\includegraphics[width=\textwidth]{appendix_figures/cityscapes_random/dp2_SGA_im288_60M_MMT_sample100_kpfix/strasbourg_000000_010816_leftImg8bit.jpg}
\includegraphics[width=\textwidth]{appendix_figures/cityscapes_random/dp2_SGA_im288_60M_MMT_sample100_kpfix/strasbourg_000000_015764_leftImg8bit.jpg}
\includegraphics[width=\textwidth]{appendix_figures/cityscapes_random/dp2_SGA_im288_60M_MMT_sample100_kpfix/stuttgart_000114_000019_leftImg8bit.jpg}
\includegraphics[width=\textwidth]{appendix_figures/cityscapes_random/dp2_SGA_im288_60M_MMT_sample100_kpfix/tubingen_000056_000019_leftImg8bit.jpg}
\includegraphics[width=\textwidth]{appendix_figures/cityscapes_random/dp2_SGA_im288_60M_MMT_sample100_kpfix/ulm_000001_000019_leftImg8bit.jpg}
\includegraphics[width=\textwidth]{appendix_figures/cityscapes_random/dp2_SGA_im288_60M_MMT_sample100_kpfix/weimar_000018_000019_leftImg8bit.jpg}
\caption{Body - Realistic (HM-LO)}
\end{subfigure}%%
\caption{Random anonymization examples from Cityscapes \cite{cityscapes}.
\textbf{HM}=Histogram matching.
\textbf{HM-LO}=Histogram matching via Latent Optimization.
Note that the images are compressed.}
\label{fig:cityscapes_random_HM_grid2}
\end{figure*}

\begin{figure*}[t]
\centering
\begin{subfigure}[t]{0.3333333333333333\textwidth}
\centering
\includegraphics[width=\textwidth]{appendix_figures/bdd100k_random/dp2_face_gaussian/00de5508-00000000.jpg}
\includegraphics[width=\textwidth]{appendix_figures/bdd100k_random/dp2_face_gaussian/0c8c70f2-160e0001.jpg}
\includegraphics[width=\textwidth]{appendix_figures/bdd100k_random/dp2_face_gaussian/0fa741ce-9b6dde95.jpg}
\includegraphics[width=\textwidth]{appendix_figures/bdd100k_random/dp2_face_gaussian/1adce148-eaba0001.jpg}
\includegraphics[width=\textwidth]{appendix_figures/bdd100k_random/dp2_face_gaussian/34eb51fe-c704575a.jpg}
\includegraphics[width=\textwidth]{appendix_figures/bdd100k_random/dp2_face_gaussian/38300e31-00000000.jpg}
\caption{Face - Gaussian}
\end{subfigure}%%
\begin{subfigure}[t]{0.3333333333333333\textwidth}
\centering
\includegraphics[width=\textwidth]{appendix_figures/bdd100k_random/dp2_face_maskout/00de5508-00000000.jpg}
\includegraphics[width=\textwidth]{appendix_figures/bdd100k_random/dp2_face_maskout/0c8c70f2-160e0001.jpg}
\includegraphics[width=\textwidth]{appendix_figures/bdd100k_random/dp2_face_maskout/0fa741ce-9b6dde95.jpg}
\includegraphics[width=\textwidth]{appendix_figures/bdd100k_random/dp2_face_maskout/1adce148-eaba0001.jpg}
\includegraphics[width=\textwidth]{appendix_figures/bdd100k_random/dp2_face_maskout/34eb51fe-c704575a.jpg}
\includegraphics[width=\textwidth]{appendix_figures/bdd100k_random/dp2_face_maskout/38300e31-00000000.jpg}
\caption{Face - Mask Out}
\end{subfigure}%%
\begin{subfigure}[t]{0.3333333333333333\textwidth}
\centering
\includegraphics[width=\textwidth]{appendix_figures/bdd100k_random/dp2_face_fdf128/00de5508-00000000.jpg}
\includegraphics[width=\textwidth]{appendix_figures/bdd100k_random/dp2_face_fdf128/0c8c70f2-160e0001.jpg}
\includegraphics[width=\textwidth]{appendix_figures/bdd100k_random/dp2_face_fdf128/0fa741ce-9b6dde95.jpg}
\includegraphics[width=\textwidth]{appendix_figures/bdd100k_random/dp2_face_fdf128/1adce148-eaba0001.jpg}
\includegraphics[width=\textwidth]{appendix_figures/bdd100k_random/dp2_face_fdf128/34eb51fe-c704575a.jpg}
\includegraphics[width=\textwidth]{appendix_figures/bdd100k_random/dp2_face_fdf128/38300e31-00000000.jpg}
\caption{Face - Realistic}
\end{subfigure}%%
\caption{Random anonymization examples from BDD100K \cite{Yu2020}.
Note that the images are compressed.}
\label{fig:bdd100k_random_grid_face0}
\end{figure*}
\begin{figure*}[t]
\centering
\begin{subfigure}[t]{0.3333333333333333\textwidth}
\centering
\includegraphics[width=\textwidth]{appendix_figures/bdd100k_random/dp2_face_gaussian/4bdd2193-546f8f2c.jpg}
\includegraphics[width=\textwidth]{appendix_figures/bdd100k_random/dp2_face_gaussian/4e767430-456e7cf7.jpg}
\includegraphics[width=\textwidth]{appendix_figures/bdd100k_random/dp2_face_gaussian/52c0315c-51a50637.jpg}
\includegraphics[width=\textwidth]{appendix_figures/bdd100k_random/dp2_face_gaussian/564397de-16d4592a.jpg}
\includegraphics[width=\textwidth]{appendix_figures/bdd100k_random/dp2_face_gaussian/5d379513-3363abb3.jpg}
\includegraphics[width=\textwidth]{appendix_figures/bdd100k_random/dp2_face_gaussian/60e2fc8e-803218f4.jpg}
\caption{Face - Gaussian}
\end{subfigure}%%
\begin{subfigure}[t]{0.3333333333333333\textwidth}
\centering
\includegraphics[width=\textwidth]{appendix_figures/bdd100k_random/dp2_face_maskout/4bdd2193-546f8f2c.jpg}
\includegraphics[width=\textwidth]{appendix_figures/bdd100k_random/dp2_face_maskout/4e767430-456e7cf7.jpg}
\includegraphics[width=\textwidth]{appendix_figures/bdd100k_random/dp2_face_maskout/52c0315c-51a50637.jpg}
\includegraphics[width=\textwidth]{appendix_figures/bdd100k_random/dp2_face_maskout/564397de-16d4592a.jpg}
\includegraphics[width=\textwidth]{appendix_figures/bdd100k_random/dp2_face_maskout/5d379513-3363abb3.jpg}
\includegraphics[width=\textwidth]{appendix_figures/bdd100k_random/dp2_face_maskout/60e2fc8e-803218f4.jpg}
\caption{Face - Mask Out}
\end{subfigure}%%
\begin{subfigure}[t]{0.3333333333333333\textwidth}
\centering
\includegraphics[width=\textwidth]{appendix_figures/bdd100k_random/dp2_face_fdf128/4bdd2193-546f8f2c.jpg}
\includegraphics[width=\textwidth]{appendix_figures/bdd100k_random/dp2_face_fdf128/4e767430-456e7cf7.jpg}
\includegraphics[width=\textwidth]{appendix_figures/bdd100k_random/dp2_face_fdf128/52c0315c-51a50637.jpg}
\includegraphics[width=\textwidth]{appendix_figures/bdd100k_random/dp2_face_fdf128/564397de-16d4592a.jpg}
\includegraphics[width=\textwidth]{appendix_figures/bdd100k_random/dp2_face_fdf128/5d379513-3363abb3.jpg}
\includegraphics[width=\textwidth]{appendix_figures/bdd100k_random/dp2_face_fdf128/60e2fc8e-803218f4.jpg}
\caption{Face - Realistic}
\end{subfigure}%%
\caption{Random anonymization examples from BDD100K \cite{Yu2020}.
Note that the images are compressed.}
\label{fig:bdd100k_random_grid_face1}
\end{figure*}
\begin{figure*}[t]
\centering
\begin{subfigure}[t]{0.3333333333333333\textwidth}
\centering
\includegraphics[width=\textwidth]{appendix_figures/bdd100k_random/dp2_face_gaussian/638f30e3-22474f13.jpg}
\includegraphics[width=\textwidth]{appendix_figures/bdd100k_random/dp2_face_gaussian/68eae8d4-3ed5f45a.jpg}
\includegraphics[width=\textwidth]{appendix_figures/bdd100k_random/dp2_face_gaussian/6a626ee3-61100bbc.jpg}
\includegraphics[width=\textwidth]{appendix_figures/bdd100k_random/dp2_face_gaussian/6ceee4e5-b52357bb.jpg}
\includegraphics[width=\textwidth]{appendix_figures/bdd100k_random/dp2_face_gaussian/734ecaa0-995f416b.jpg}
\includegraphics[width=\textwidth]{appendix_figures/bdd100k_random/dp2_face_gaussian/7c67d03c-c77e4d7a.jpg}
\caption{Face - Gaussian}
\end{subfigure}%%
\begin{subfigure}[t]{0.3333333333333333\textwidth}
\centering
\includegraphics[width=\textwidth]{appendix_figures/bdd100k_random/dp2_face_maskout/638f30e3-22474f13.jpg}
\includegraphics[width=\textwidth]{appendix_figures/bdd100k_random/dp2_face_maskout/68eae8d4-3ed5f45a.jpg}
\includegraphics[width=\textwidth]{appendix_figures/bdd100k_random/dp2_face_maskout/6a626ee3-61100bbc.jpg}
\includegraphics[width=\textwidth]{appendix_figures/bdd100k_random/dp2_face_maskout/6ceee4e5-b52357bb.jpg}
\includegraphics[width=\textwidth]{appendix_figures/bdd100k_random/dp2_face_maskout/734ecaa0-995f416b.jpg}
\includegraphics[width=\textwidth]{appendix_figures/bdd100k_random/dp2_face_maskout/7c67d03c-c77e4d7a.jpg}
\caption{Face - Mask Out}
\end{subfigure}%%
\begin{subfigure}[t]{0.3333333333333333\textwidth}
\centering
\includegraphics[width=\textwidth]{appendix_figures/bdd100k_random/dp2_face_fdf128/638f30e3-22474f13.jpg}
\includegraphics[width=\textwidth]{appendix_figures/bdd100k_random/dp2_face_fdf128/68eae8d4-3ed5f45a.jpg}
\includegraphics[width=\textwidth]{appendix_figures/bdd100k_random/dp2_face_fdf128/6a626ee3-61100bbc.jpg}
\includegraphics[width=\textwidth]{appendix_figures/bdd100k_random/dp2_face_fdf128/6ceee4e5-b52357bb.jpg}
\includegraphics[width=\textwidth]{appendix_figures/bdd100k_random/dp2_face_fdf128/734ecaa0-995f416b.jpg}
\includegraphics[width=\textwidth]{appendix_figures/bdd100k_random/dp2_face_fdf128/7c67d03c-c77e4d7a.jpg}
\caption{Face - Realistic}
\end{subfigure}%%
\caption{Random anonymization examples from BDD100K \cite{Yu2020}.
Note that the images are compressed.}
\label{fig:bdd100k_random_grid_face2}
\end{figure*}
\begin{figure*}[t]
\centering
\begin{subfigure}[t]{0.3333333333333333\textwidth}
\centering
\includegraphics[width=\textwidth]{appendix_figures/bdd100k_random/dp2_face_gaussian/7fe43deb-5d021fd3.jpg}
\includegraphics[width=\textwidth]{appendix_figures/bdd100k_random/dp2_face_gaussian/830c6cb2-f7b30a4c.jpg}
\includegraphics[width=\textwidth]{appendix_figures/bdd100k_random/dp2_face_gaussian/ad0b7d33-16243e40.jpg}
\caption{Face - Gaussian}
\end{subfigure}%%
\begin{subfigure}[t]{0.3333333333333333\textwidth}
\centering
\includegraphics[width=\textwidth]{appendix_figures/bdd100k_random/dp2_face_maskout/7fe43deb-5d021fd3.jpg}
\includegraphics[width=\textwidth]{appendix_figures/bdd100k_random/dp2_face_maskout/830c6cb2-f7b30a4c.jpg}
\includegraphics[width=\textwidth]{appendix_figures/bdd100k_random/dp2_face_maskout/ad0b7d33-16243e40.jpg}
\caption{Face - Mask Out}
\end{subfigure}%%
\begin{subfigure}[t]{0.3333333333333333\textwidth}
\centering
\includegraphics[width=\textwidth]{appendix_figures/bdd100k_random/dp2_face_fdf128/7fe43deb-5d021fd3.jpg}
\includegraphics[width=\textwidth]{appendix_figures/bdd100k_random/dp2_face_fdf128/830c6cb2-f7b30a4c.jpg}
\includegraphics[width=\textwidth]{appendix_figures/bdd100k_random/dp2_face_fdf128/ad0b7d33-16243e40.jpg}
\caption{Face - Realistic}
\end{subfigure}%%
\caption{Random anonymization examples from BDD100K \cite{Yu2020}.
Note that the images are compressed.}
\label{fig:bdd100k_random_grid_face3}
\end{figure*}

\begin{figure*}[t]
\centering
\begin{subfigure}[t]{0.3333333333333333\textwidth}
\centering
\includegraphics[width=\textwidth]{appendix_figures/bdd100k_random/dp2_body_gaussian/00de5508-00000000.jpg}
\includegraphics[width=\textwidth]{appendix_figures/bdd100k_random/dp2_body_gaussian/0c8c70f2-160e0001.jpg}
\includegraphics[width=\textwidth]{appendix_figures/bdd100k_random/dp2_body_gaussian/0fa741ce-9b6dde95.jpg}
\includegraphics[width=\textwidth]{appendix_figures/bdd100k_random/dp2_body_gaussian/1adce148-eaba0001.jpg}
\includegraphics[width=\textwidth]{appendix_figures/bdd100k_random/dp2_body_gaussian/34eb51fe-c704575a.jpg}
\includegraphics[width=\textwidth]{appendix_figures/bdd100k_random/dp2_body_gaussian/38300e31-00000000.jpg}
\caption{Body - Gaussian}
\end{subfigure}%%
\begin{subfigure}[t]{0.3333333333333333\textwidth}
\centering
\includegraphics[width=\textwidth]{appendix_figures/bdd100k_random/dp2_body_maskout/00de5508-00000000.jpg}
\includegraphics[width=\textwidth]{appendix_figures/bdd100k_random/dp2_body_maskout/0c8c70f2-160e0001.jpg}
\includegraphics[width=\textwidth]{appendix_figures/bdd100k_random/dp2_body_maskout/0fa741ce-9b6dde95.jpg}
\includegraphics[width=\textwidth]{appendix_figures/bdd100k_random/dp2_body_maskout/1adce148-eaba0001.jpg}
\includegraphics[width=\textwidth]{appendix_figures/bdd100k_random/dp2_body_maskout/34eb51fe-c704575a.jpg}
\includegraphics[width=\textwidth]{appendix_figures/bdd100k_random/dp2_body_maskout/38300e31-00000000.jpg}
\caption{Body - Mask Out}
\end{subfigure}%%
\begin{subfigure}[t]{0.3333333333333333\textwidth}
\centering
\includegraphics[width=\textwidth]{appendix_figures/bdd100k_random/dp2_SGA_im288_60M_MMT_kpfix/00de5508-00000000.jpg}
\includegraphics[width=\textwidth]{appendix_figures/bdd100k_random/dp2_SGA_im288_60M_MMT_kpfix/0c8c70f2-160e0001.jpg}
\includegraphics[width=\textwidth]{appendix_figures/bdd100k_random/dp2_SGA_im288_60M_MMT_kpfix/0fa741ce-9b6dde95.jpg}
\includegraphics[width=\textwidth]{appendix_figures/bdd100k_random/dp2_SGA_im288_60M_MMT_kpfix/1adce148-eaba0001.jpg}
\includegraphics[width=\textwidth]{appendix_figures/bdd100k_random/dp2_SGA_im288_60M_MMT_kpfix/34eb51fe-c704575a.jpg}
\includegraphics[width=\textwidth]{appendix_figures/bdd100k_random/dp2_SGA_im288_60M_MMT_kpfix/38300e31-00000000.jpg}
\caption{Body - Realistic}
\end{subfigure}%%
\caption{Random anonymization examples from BDD100K \cite{Yu2020}.
Note that the images are compressed.}
\label{fig:bdd100k_random_grid_body0}
\end{figure*}
\begin{figure*}[t]
\centering
\begin{subfigure}[t]{0.3333333333333333\textwidth}
\centering
\includegraphics[width=\textwidth]{appendix_figures/bdd100k_random/dp2_body_gaussian/4bdd2193-546f8f2c.jpg}
\includegraphics[width=\textwidth]{appendix_figures/bdd100k_random/dp2_body_gaussian/4e767430-456e7cf7.jpg}
\includegraphics[width=\textwidth]{appendix_figures/bdd100k_random/dp2_body_gaussian/52c0315c-51a50637.jpg}
\includegraphics[width=\textwidth]{appendix_figures/bdd100k_random/dp2_body_gaussian/564397de-16d4592a.jpg}
\includegraphics[width=\textwidth]{appendix_figures/bdd100k_random/dp2_body_gaussian/5d379513-3363abb3.jpg}
\includegraphics[width=\textwidth]{appendix_figures/bdd100k_random/dp2_body_gaussian/60e2fc8e-803218f4.jpg}
\caption{Body - Gaussian}
\end{subfigure}%%
\begin{subfigure}[t]{0.3333333333333333\textwidth}
\centering
\includegraphics[width=\textwidth]{appendix_figures/bdd100k_random/dp2_body_maskout/4bdd2193-546f8f2c.jpg}
\includegraphics[width=\textwidth]{appendix_figures/bdd100k_random/dp2_body_maskout/4e767430-456e7cf7.jpg}
\includegraphics[width=\textwidth]{appendix_figures/bdd100k_random/dp2_body_maskout/52c0315c-51a50637.jpg}
\includegraphics[width=\textwidth]{appendix_figures/bdd100k_random/dp2_body_maskout/564397de-16d4592a.jpg}
\includegraphics[width=\textwidth]{appendix_figures/bdd100k_random/dp2_body_maskout/5d379513-3363abb3.jpg}
\includegraphics[width=\textwidth]{appendix_figures/bdd100k_random/dp2_body_maskout/60e2fc8e-803218f4.jpg}
\caption{Body - Mask Out}
\end{subfigure}%%
\begin{subfigure}[t]{0.3333333333333333\textwidth}
\centering
\includegraphics[width=\textwidth]{appendix_figures/bdd100k_random/dp2_SGA_im288_60M_MMT_kpfix/4bdd2193-546f8f2c.jpg}
\includegraphics[width=\textwidth]{appendix_figures/bdd100k_random/dp2_SGA_im288_60M_MMT_kpfix/4e767430-456e7cf7.jpg}
\includegraphics[width=\textwidth]{appendix_figures/bdd100k_random/dp2_SGA_im288_60M_MMT_kpfix/52c0315c-51a50637.jpg}
\includegraphics[width=\textwidth]{appendix_figures/bdd100k_random/dp2_SGA_im288_60M_MMT_kpfix/564397de-16d4592a.jpg}
\includegraphics[width=\textwidth]{appendix_figures/bdd100k_random/dp2_SGA_im288_60M_MMT_kpfix/5d379513-3363abb3.jpg}
\includegraphics[width=\textwidth]{appendix_figures/bdd100k_random/dp2_SGA_im288_60M_MMT_kpfix/60e2fc8e-803218f4.jpg}
\caption{Body - Realistic}
\end{subfigure}%%
\caption{Random anonymization examples from BDD100K \cite{Yu2020}.
Note that the images are compressed.}
\label{fig:bdd100k_random_grid_body1}
\end{figure*}
\begin{figure*}[t]
\centering
\begin{subfigure}[t]{0.3333333333333333\textwidth}
\centering
\includegraphics[width=\textwidth]{appendix_figures/bdd100k_random/dp2_body_gaussian/638f30e3-22474f13.jpg}
\includegraphics[width=\textwidth]{appendix_figures/bdd100k_random/dp2_body_gaussian/68eae8d4-3ed5f45a.jpg}
\includegraphics[width=\textwidth]{appendix_figures/bdd100k_random/dp2_body_gaussian/6a626ee3-61100bbc.jpg}
\includegraphics[width=\textwidth]{appendix_figures/bdd100k_random/dp2_body_gaussian/6ceee4e5-b52357bb.jpg}
\includegraphics[width=\textwidth]{appendix_figures/bdd100k_random/dp2_body_gaussian/734ecaa0-995f416b.jpg}
\includegraphics[width=\textwidth]{appendix_figures/bdd100k_random/dp2_body_gaussian/7c67d03c-c77e4d7a.jpg}
\caption{Body - Gaussian}
\end{subfigure}%%
\begin{subfigure}[t]{0.3333333333333333\textwidth}
\centering
\includegraphics[width=\textwidth]{appendix_figures/bdd100k_random/dp2_body_maskout/638f30e3-22474f13.jpg}
\includegraphics[width=\textwidth]{appendix_figures/bdd100k_random/dp2_body_maskout/68eae8d4-3ed5f45a.jpg}
\includegraphics[width=\textwidth]{appendix_figures/bdd100k_random/dp2_body_maskout/6a626ee3-61100bbc.jpg}
\includegraphics[width=\textwidth]{appendix_figures/bdd100k_random/dp2_body_maskout/6ceee4e5-b52357bb.jpg}
\includegraphics[width=\textwidth]{appendix_figures/bdd100k_random/dp2_body_maskout/734ecaa0-995f416b.jpg}
\includegraphics[width=\textwidth]{appendix_figures/bdd100k_random/dp2_body_maskout/7c67d03c-c77e4d7a.jpg}
\caption{Body - Mask Out}
\end{subfigure}%%
\begin{subfigure}[t]{0.3333333333333333\textwidth}
\centering
\includegraphics[width=\textwidth]{appendix_figures/bdd100k_random/dp2_SGA_im288_60M_MMT_kpfix/638f30e3-22474f13.jpg}
\includegraphics[width=\textwidth]{appendix_figures/bdd100k_random/dp2_SGA_im288_60M_MMT_kpfix/68eae8d4-3ed5f45a.jpg}
\includegraphics[width=\textwidth]{appendix_figures/bdd100k_random/dp2_SGA_im288_60M_MMT_kpfix/6a626ee3-61100bbc.jpg}
\includegraphics[width=\textwidth]{appendix_figures/bdd100k_random/dp2_SGA_im288_60M_MMT_kpfix/6ceee4e5-b52357bb.jpg}
\includegraphics[width=\textwidth]{appendix_figures/bdd100k_random/dp2_SGA_im288_60M_MMT_kpfix/734ecaa0-995f416b.jpg}
\includegraphics[width=\textwidth]{appendix_figures/bdd100k_random/dp2_SGA_im288_60M_MMT_kpfix/7c67d03c-c77e4d7a.jpg}
\caption{Body - Realistic}
\end{subfigure}%%
\caption{Random anonymization examples from BDD100K \cite{Yu2020}.
Note that the images are compressed.}
\label{fig:bdd100k_random_grid_body2}
\end{figure*}
\begin{figure*}[t]
\centering
\begin{subfigure}[t]{0.3333333333333333\textwidth}
\centering
\includegraphics[width=\textwidth]{appendix_figures/bdd100k_random/dp2_body_gaussian/7fe43deb-5d021fd3.jpg}
\includegraphics[width=\textwidth]{appendix_figures/bdd100k_random/dp2_body_gaussian/830c6cb2-f7b30a4c.jpg}
\includegraphics[width=\textwidth]{appendix_figures/bdd100k_random/dp2_body_gaussian/ad0b7d33-16243e40.jpg}
\caption{Body - Gaussian}
\end{subfigure}%%
\begin{subfigure}[t]{0.3333333333333333\textwidth}
\centering
\includegraphics[width=\textwidth]{appendix_figures/bdd100k_random/dp2_body_maskout/7fe43deb-5d021fd3.jpg}
\includegraphics[width=\textwidth]{appendix_figures/bdd100k_random/dp2_body_maskout/830c6cb2-f7b30a4c.jpg}
\includegraphics[width=\textwidth]{appendix_figures/bdd100k_random/dp2_body_maskout/ad0b7d33-16243e40.jpg}
\caption{Body - Mask Out}
\end{subfigure}%%
\begin{subfigure}[t]{0.3333333333333333\textwidth}
\centering
\includegraphics[width=\textwidth]{appendix_figures/bdd100k_random/dp2_SGA_im288_60M_MMT_kpfix/7fe43deb-5d021fd3.jpg}
\includegraphics[width=\textwidth]{appendix_figures/bdd100k_random/dp2_SGA_im288_60M_MMT_kpfix/830c6cb2-f7b30a4c.jpg}
\includegraphics[width=\textwidth]{appendix_figures/bdd100k_random/dp2_SGA_im288_60M_MMT_kpfix/ad0b7d33-16243e40.jpg}
\caption{Body - Realistic}
\end{subfigure}%%
\caption{Random anonymization examples from BDD100K \cite{Yu2020}.
Note that the images are compressed.}
\label{fig:bdd100k_random_grid_body3}
\end{figure*}
